# Supplementary material for: Parameterized Broadcast Networks with Registers: from NP to the Frontiers of Decidability
Source: arXiv:2306.01517 source file (2024-03-04)
Supplement: Supplementary file 1 [file Preuve-simple-protocols.tex]

\section{Proof of Proposition~\ref{prop:loc-eq-test-elimination}}
\label{sec:proof-lol-eq-test-elim}

\SimpleReduction*

\begin{proof}
	We construct a "protocol" $\prot'$ with no "local equality tests" so that any "initial run" of $\prot$ may be turned into an "initial run" of $\prot'$ and vice-versa. 
	The intuition is as follows. $\prot'$ corresponds to $\prot$, where an abstract layer is added in the treatments of the registers. In $\prot'$, we do not directly store each register but rather equality relations between them, so that a value shared by several registers is only stored once. We dub registers of $\prot'$ ""memory slots"" to distinguish them from the registers of $\prot$. A "memory slot" will be used to store a value shared between registers. 
	We will need $\regnum$ "memory slots" to do so. Moreover, we will need a mapping $\map : \nset{1}{r} \to \nset{1}{r}$ that tells, for each register, in which "memory slot" its value is stored. This mapping will be directly encoded in the set of states of $\prot'$, which causes an exponential blow-up in the "size" of the "protocol".
	
	For simplicity, we allow our "protocol" $\prot'$ to have dummy transitions with no effect (such transitions can be encoded using broadcasts with a dummy "message type"). 
	
	Let $\prot = (Q, \messages, \transitions, q_0, \regnum)$. 
	We define $\prot' := (Q', \messages, \transitions', q_0', \regnum)$ as follows. The set of states is $Q' := Q \times (\nset{1}{r} \to \nset{1}{r})$, its initial state is $q_0' := (q_0, \idmap)$ where $\idmap(i) = i$ for all $i \in \nset{1}{r}$. 
	
	The set of transitions $\transitions'$ is defined as follows.
	$\prot'$ mimics the operations of $\prot$ step-by-step. When $\prot$ stores a new value, $\prot'$ guesses whether this value is already stored in one of the "memory slots" (then it simply checks that the received value is the one of that "memory slot" with a $\rec{m}{i}{\eqtestact}$) or is not stored yet (then it stores it in an empty "memory slot"). In both cases it updates the mapping accordingly.
	Formally, for all $q,q' \in Q$ and $\map, \map' \in \nset{1}{r} \to \nset{1}{r}$, we have $((q, \map), \op, (q', \map')) \in \transitions'$ in the following cases:
	
	\begin{itemize}
		\item $\op = \br{m}{j}$, 
		$\map = \map'$ and $(q, \br{m}{i}, q') \in \transitions$ for some $i$ such that $\map(i) = j$ (we broadcast the value stored in the corresponding "memory slot").
		
		\item $\op=\rec{m}{j}{\enregact}$, there is a transition $(q, \rec{m}{i_0}{\enregact}, q') \in \transitions$ with $\map^{-1}(j) \subseteq \set{i_0}$ and for all $i \in \nset{1}{r}$, if $i \ne i_0$ then $\map'(i) = \map(i)$ and $\map'(i_0) = j$ (the received value is stored into a fresh "memory slot").
		
		\item $\op = \rec{m}{j}{\eqtestact}$ and either
		\begin{itemize}
			\item there is a transition $(q, \rec{m}{i}{\eqtestact}, q') \in \transitions$ such that $\map(i)=j$ and $\map'=\map$ (to test equality with register $i$, we test equality with the "memory slot" containing value of register $i$), or
			
			\item there is a transition $(q, \rec{m}{i_0}{\enregact}, q') \in \transitions$ such that $\map'(i_0)=j$ and $\map'(i) = \map(i)$ for every $i \neq i_0$ (register $i_0$ stores a value that is guessed as being already in a "memory slot" hence we simply modify the mapping).
		\end{itemize} 
		
		\item $\op = \rec{m}{j}{\diseqtestact}$ and there is a transition $(q, \rec{m}{i}{\diseqtestact}, q') \in \transitions$ such that $\map(i)=j$ (to test disequality with register $i$, we test disequality with the "memory slot" containing value of register $i$).

		\item $\op=\loc{j_1}{j_2}{\diseqtestact}$ and there is a transition $(q, \loc{i_1}{i_2}{\diseqtestact}, q')$ such that $\map(i_1)=j_1$ and $\map(i_2) = j_2$ (to implement a local disequality test, we do the corresponding test on "memory slots"; this test always fails if $j_1 = j_2$).

		\item $\op = \rec{m}{j}{\dummyact}$ and there is a transition $(q, \rec{m}{i}{\dummyact}, q') \in \transitions$ for some $i \in \nset{1}{r}$.
	\end{itemize}
	
	Additionally, there is a dummy transition between $(q,\map)$ and $(q',\map')$ whenever there exist $i_1, i_2$ such that $(q, \loc{i_1}{i_2}{\eqtestact}, q') \in \transitions$ and $\map(i_1) = \map(i_2)$ (an equality test on two registers mapped to the same "memory slot" automatically succeeds).

	Note that we cannot in fact guarantee that values stored in the "memory slots" are all distinct, because, upon reception of a value, we may only perform one test and therefore cannot test that the value is different from all stored values. This is why we still need "local disequality tests" in $\prot'$. In practice, when a agent in $\prot$ performs a $\quotemarks{\enregact}$ reception of a broadcast with a value that is already in one of its "memory slots", the corresponding agent in $\prot'$ may non-deterministically notice that it already has this value in a "memory slot" (corresponds to a $\rec{\amessage}{j}{\eqtestact}$ transition) but it may also store it in a fresh "memory slot" (corresponds to a $\rec{\amessage}{j}{\enregact}$ transition). Therefore, the encoding of the content of the registers into a mapping and "memory slots" is not unique, even up to permutation of the "memory slots". However, encodings that do not gather together registers with the same value will simply allow less transitions (it will forbid some equality tests), therefore this is not an issue. 

	We now prove that, for a given state $q_f \in Q$, $q_f$ may be covered in $\prot$ if and only if some state of $Q_f' := \set{(q_f, \map) \mid \map \in \nset{1}{r} \to \nset{1}{r}}$ may be covered in $\prot'$. To do so, we will prove that any "initial run" of $\prot$ may be turned into an "initial run" of $\prot'$ and vice-versa. 
  
	Let $\agents \subseteq \nats$.
	Given a configuration $\config$ of $\prot$, we denote by \AP $\intro*\memoryproj{\config}$ 
	the set of configurations $\config'$ over $\agents$ such that:
	 for all $a \in \agents$, by denoting $(q, \localdata):= \config(a)$, one has $\config'(a) = ((q, \map), \localdata')$ where, for every $i \in \nset{1}{r}$, $\localdata'(\map(i)) = \localdata(i)$. 
	Moreover, we denote by $\intro*\perfproj{\config}$ 
	the subset of $\memoryproj{\config}$ containing configurations 
	$\config'$ that additionally satisfy that, for every agent, for every $j \ne j' \in \nset{1}{r}$, $\localdata'(j) \ne \localdata'(j')$ (we call such configurations ""perfect configurations"" of $\prot'$).

	Let $\run: \config_0 \step{*} \config_f$ an "initial run" on $\prot$ over some set of agents $\agents$. We prove by induction on the length of $\run$ that there exists an "initial run" $\run': \config_0' \step{*} \config_f'$ on $\prot'$ over $\agents$ such that $\config_f' \in \perfproj{\config_f}$. This property is trivially true for $\run$ of length $0$. It therefore suffices to prove that given $\config_1 \step{} \config_2$ and $\config_1' \in \perfproj{\config_1}$, there exists $\config_2' \in \perfproj{\config_2}$ such that $\config_1' \step{} \config_2'$. We denote by $s$ the "step" $\config_1 \step{} \config_2$ and by $s'$ the "step" $\config'_1 \step{} \config'_2$ that we are building. 
	Let $a \in \agents$ that performs a transition in $s$.
	\begin{itemize}
	\item If $a$ performs a local test $\loc{i_1}{i_2}{\diseqtestact}$ in $s$, then it may perform the corresponding local test in $s'$ because $\config_1' \in \memoryproj{\config_1}$ hence $\config_1'(a)$ maps $i_1$ and $i_2$ to "memory slots" of distinct values. 
	\item If $a$ performs a local test  $\loc{i_1}{i_2}{\eqtestact}$, then because $\config_1'\in \perfproj{\config_1}$, it maps $i_1$ and $i_2$ to the same "memory slot" and $a$ may perform the corresponding internal transition in $\prot'$.  
	\item If $a$ performs a broadcast in $s$, then we make it perform the corresponding broadcast in $s'$. Note that, because $\config_1' \in \memoryproj{\config_1}$, the broadcast value is the same in $s$ and $s'$. 
	\item 
	Suppose now that $a$ performs a reception $\rec{\amessage}{i}{\anact}$ in $s$. Let $\aval$ the value of the message. By the previous case, the corresponding broadcast is performed in $s'$ with the same value $\aval$. 
		\begin{itemize}
		\item If $\anact = \quotemarks{\dummyact}$, then we make $a$ perform the corresponding transition in $s'$. 
		\item If $\anact = \quotemarks{\enregact}$, then if $\aval$ appears in some "memory slot" $j$ in $\config_1'$, we make $a$ perform the corresponding $\rec{\amessage}{j}{\eqtestact}$ transition in $s'$. 
		If $\aval$ does not appear in any "memory slot", then we make $a$ take the $\rec{\amessage}{j}{\enregact}$ transition with $j$ a "memory slot" that did not store the value of any register other that $i$ (it necessarily exists by the pigeonhole principle). This case disjunction guarantees that $\config_2'(a)$ does not have twice the same value in its "memory slots", hence that $\config_2'$ is "perfect".
		\item If $\anact = \quotemarks{\diseqtestact}$, then we make $a$ perform the corresponding transition in $s'$ with the operation $\rec{m}{\map(j)}{\diseqtestact}$; because $\config_1' \in \memoryproj{\config_1}$,  we have $\config_1'(a)(\map(j)) = \config_1(a)(j) \ne v$ and the test passes.
		\item If $\anact = \quotemarks{\diseqtestact}$, then we make $a$ perform the corresponding transition in $s'$ with the operation $\rec{m}{\map(j)}{\eqtestact}$; because $\config_1' \in \memoryproj{\config_1}$,  we have $\config_1'(a)(\map(j)) = \config_1(a)(j) = v$ and the test passes.	
		\end{itemize}
	\end{itemize}

	Overall, we have built $\config_2' \in \perfproj{\config_2}$ such that $\config_1' \step{} \config_2'$ in $\prot'$, which concludes the induction. We have proven that for every $\run: \config_0 \step{*} \config_f$ there exists $\run': \config_0' \step{*} \config_f'$ on $\prot'$ such that $\config_f' \in \perfproj{\config_f}$. This proves that if $q_f$ may be covered in $\prot$, then $Q_f'$ may be covered in $\prot'$. 

	Conversely, let $\run' : \config_0' \step{*} \config_f'$ an "initial run" of $\prot$ over some set of agents $\agents$. We prove that there exists an "initial run" $\run: \config_0 \step{*} \config_f$ of $\prot$ such that $\config_f' \in \memoryproj{\config_f}$. The proof is by induction on the length of $\run'$. 

	For $\run'$ of length $0$, the property is trivially satisfied. For the heredity, it suffices to prove that if we are given $\config_1' \step{} \config_2'$ and $\config_1$ such that $\config_1' \in \memoryproj{\config_1}$, then there exists $\config_2$ such that $\config_2' \in \memoryproj{\config_2}$ and $\config_1 \step{} \config_2$. The proof is similar to the previous one but simpler. Let $a$ an agent. We pick $\atrans \in \transitions$ one of the transitions in $\prot$ that, when building $\prot'$, caused the transition taken by $a$ in $\config_1' \step{} \config_2'$ to be added to $\transitions'$. A simple case disjunction allows to prove that $a$ may perform $\atrans$ from $\config_1$ (under the assumption that the broadcast value is the same, which can be easily guaranteed by looking at the broadcasting agent). Overall we obtain a "step" $\config_1 \step{} \config_2$ with $\config_2' \in \memoryproj{\config_2}$ by construction. This concludes the induction. We have proven that if $Q_f'$ can be covered in $\prot'$ then $q_f$ can be covered in $\prot$, hence the two properties are equivalent.
	Finally, observe that the \COVER problem with a subset $Q_f' \subseteq Q'$ as objective can be easily reduced to \COVER with a single state as objective (using dummy transitions with no effect) concluding the reduction.
\end{proof}
